# Supplementary material for: $\mathcal{PT}$-Symmetric Topological Edge-Gain Effect
Source: arXiv:1910.10946 source file (2020-07-10)
Supplement: Supplementary file 1 [file supplementary_v13_a.pdf]

# Supplementary information for
# $\mathcal{PT}$-symmetric topological edge-gain effect

Alex Y. Song,[1] Xiao-Qi Sun,[2] Avik Dutt,[1] Momchil Minkov,[1] Casey Wojcik,[1]
Haiwen Wang,[3] Ian Williamson,[1] Meir Orenstein,[4] and Shanhui Fan[1,*]

[1]*Department of Electrical Engineering,*
*Stanford University, Stanford, CA94305, USA*

[2]*Department of Physics, Stanford University, Stanford, CA94305, USA*

[3]*Department of Applied Physics, Stanford University, Stanford, CA94305, USA*

[4]*Department of Electrical Engineering,*
*Technion - Israel Institute of Technology,*
*Technion City, Haifa 3200003, Israel*

(Dated: 9th July 2020)

## GENERAL RECIPE FOR NON-HERMITIAN COUPLINGS

Suppose we start with a quantum spin hall (QSH) system with inversion and time reversal symmetry, described by the following Hermitian Hamiltonian in the momentum space

$$H(k) = \begin{pmatrix} h_\uparrow(k) & 0 \\ 0 & h_\downarrow(k) \end{pmatrix} \tag{1}$$

Here, $h_\uparrow$ and $h_\downarrow$ are the Hamiltonians for the two spins, respectively.

It is known that the band structure of a system with time reversal and inversion symmetry is two-fold degenerate. Here we explicitly construct the degenerate states at any $k$. We first realize that for a time-reversal system, we must have $h_\downarrow(k) = h_\uparrow^*(-k)$. Here the time reversal operator is $\mathcal{T} = i\sigma_y \otimes I K_0$, where $\sigma_i$ is a Pauli matrix, and $K_0$ is the complex conjugation. In the following, we denote $h(k) \triangleq h_\uparrow(k) = h_\downarrow^*(-k)$.

At any momentum $k$, we assume there is a state $|\psi(k)\rangle$ with energy $E(k)$ for the up-spin, i.e. $h(k)\,|\psi(k)\rangle = E(k)\,|\psi(k)\rangle$. By inversion symmetry, there must be a spin-up state at $-k$ with the same energy, i.e. $h(-k)\,|\psi(-k)\rangle = E(k)\,|\psi(-k)\rangle$. It follows that $h^*(-k)\,|\psi^*(-k)\rangle = E(k)\,|\psi^*(-k)\rangle$. Since $h_\downarrow(k) = h^*(-k)$, we have found the down-spin state with energy $E(k)$. We denote this state as $|\varphi(k)\rangle = |\psi^*(-k)\rangle$. Therefore, at every k the eigenstates of $H(k)$ are two-fold degenerate, with the form:

$$|\psi_1(k)\rangle = \begin{pmatrix} |\psi(k)\rangle \\ 0 \end{pmatrix}, \quad |\psi_2(k)\rangle = \begin{pmatrix} 0 \\ |\varphi(k)\rangle \end{pmatrix} \tag{2}$$

### The recipe

We now add to the Hamiltonian of Eq. (1) an additional non-Hermitian coupling matrix

$$\Gamma(k) = \begin{pmatrix} 0 & f_1(k)\kappa(k) \\ f_2(k)\kappa(k) & 0 \end{pmatrix}, \quad \kappa(k) = h_\uparrow(k) - h_\downarrow(k) \tag{3}$$

Here $f_1(k)$ and $f_2(k)$ are complex functions with the only constraint that $f_1(k)f_2(k)$ is real.

We first show that $\Gamma$ does not couple the two degenerate states, i.e. Eq. (2), of the system. For a pair of degenerate states shown in Eq. (2), it is straightforward to verify that $\langle\psi(k)|\,(h(k) - h^*(-k))\,|\varphi(k)\rangle = 0$. It follows that $\langle\psi_1|\,\Gamma\,|\psi_2\rangle = 0$.

Next, we show that $H+\Gamma$ satisfies pseudo-Hermiticity, which guarantees its eigenenergies are either real or complex conjugate pairs [1–4]. We will prove this at each $k$ independently. For simplicity, in the following we suppress the $k$ index.

The definition of pseudo-Hermiticity is reproduced as follows. For a matrix $M$, if there exists an Hermitian matrix $\mathcal{P}$ such that $\mathcal{P}M\mathcal{P}^{-1} = M^{\dagger}$ where $M^{\dagger}$ means the Hermitian conjugate of $M$, then we say matrix $M$ is $\mathcal{P}$-pseudo-Hermitian [1]. It has been shown that if a matrix is pseudo-Hermitian, then its eigen spectrum must be either real or complex conjugate pairs [1].

We will prove a slightly more general form than Eq. (3), as follows. Suppose $h_1$ and $h_2$ are two Hermitian Hamiltonians of dimension $m \times m$ and $n \times n$, respectively. $\kappa$ is an $m \times n$ general complex matrix, and $f_1$ and $f_2$ are two complex numbers such that $f_1 f_2$ is a real number. Then it is straightforward to show the following non-Hermitian Hamiltonian

$$\mathcal{H} = \begin{pmatrix} h_1 & f_1\kappa \\ f_2\kappa^{\dagger} & h_2 \end{pmatrix} \tag{4}$$

satisfies $\mathcal{P}$-pseudo-Hermiticity, with the following operator $\mathcal{P}$:

$$\mathcal{P} = \begin{pmatrix} |f_2| I_{m\times m} & 0 \\ 0 & s|f_1| I_{n\times n} \end{pmatrix} \tag{5}$$

where $s = \mathrm{sgn}(f_1 f_2)$.

Since $h_{\uparrow}, h_{\downarrow}, \kappa$ are all Hermitian matrices, $H + \Gamma$ is a special case of Eq. (4). Thus the general recipe does lead to a pseudo-Hermitian system where the eigenvalues are either real or complex conjugate pairs.

**General systems without time reversal or inversion symmetry**

Here we generalize the discussions above to a QSH-like system without time-reversal or inversion symmetry. We consider a general system which consists of two sub-systems, described by the Hamiltonian in Eq. (1), which is reproduced here:

$$H = \begin{pmatrix} h_{\uparrow} & 0 \\ 0 & h_{\downarrow} \end{pmatrix} \tag{6}$$

Here the notation $\uparrow$ and $\downarrow$ merely identify the two subsystems, and are not necessarily two spins. We again have suppressed the $k$ index, since the discussion is carried out at each $k$

independently. We denote the eigen states of $h_\uparrow$ and $h_\downarrow$ by $|s, \mu\rangle$, where $s$ represents the two subsystems $\uparrow$ and $\downarrow$, and $\mu$ is the index of the eigenstates. We assume the $\mu$'th state of the two subsystems lie within the same energy range, and there is a gap between different bands with different $\mu$.

We now consider the following non-Hermitian coupling matrix $\Gamma$,

$$\Gamma = \begin{pmatrix} 0 & f_1 \kappa \\ f_2 \kappa^\dagger & 0 \end{pmatrix}, \quad \kappa = \sum_{i \neq j} |\uparrow i\rangle \langle \downarrow j| \tag{7}$$

Here, $f_1$ and $f_2$ are complex numbers such that $f_1 f_2$ is real. This coupling matrix provides the topological edge-gain effect. It is clear that $\Gamma$ does not couple states within the same subsystem by construction. Moreover, since the Hamiltonian $H + \Gamma$ satisfies the form of Eq. (4), it satisfies pseudo-Hermiticity, and hence its eigenenergies must be either real or complex pairs. We note that $\Gamma$ does not couple two states of the same index $\mu$ in different subsystems , which is a necessary condition for the bulk to be in the $\mathcal{PT}$ exact phase. It is also noted that the construction in Eq. (6) and Eq. (7) is regardless of the physical dimension of the system.

## EFFECTIVE $2 \times 2$ HAMILTONIAN NEAR THE EDGE CROSSING

A $2 \times 2$ effective Hamiltonian can be obtained for the edge states of the topological edge-gain models. Generically, we start with a crossing of two edge bands, each to the lowest order has a linear dispersion near the crossing point. Such crossing and degeneracy do not require any symmetry in the system but are guaranteed by the bulk topology. The non-Hermitian coupling will induce a coupling between the two edge bands. This coupling could have a wavevector dependence in general but its lowest order can be a constant. We hence arrive at the following $2 \times 2$ effective Hamiltonian in the vicinity of the crossing point:

$$H_{eff} = \begin{pmatrix} \omega_0 + \alpha k & i\gamma' \\ i\gamma' & \omega_0 + \beta k \end{pmatrix} \tag{8}$$

where the slope of the two bands $\alpha, \beta$ can be calculated by the underlying Hermitian model before the introduction of the non-Hermitian coupling. The non-Hermitian coupling strength $i\gamma'$ can be obtained either analytically or by numerical fitting.

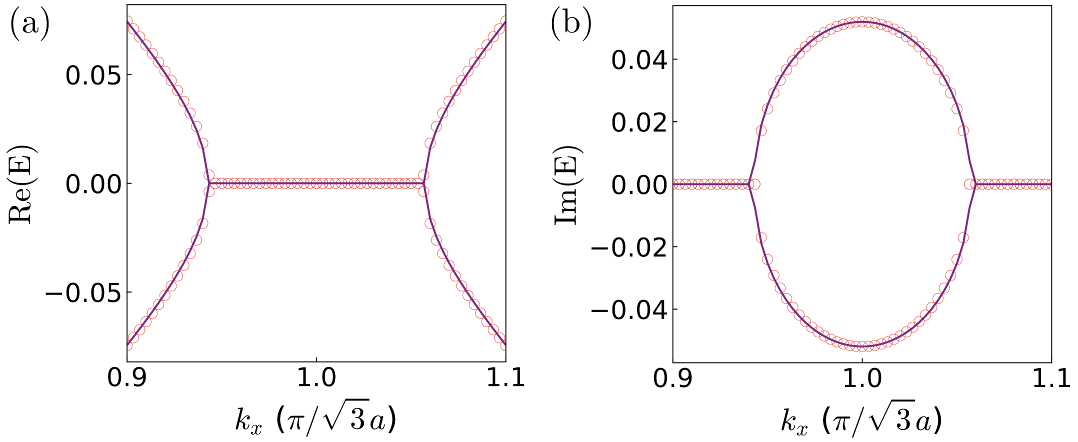


Figure 1. The (a) real part and the (b) imaginary part of the edge bands in Kane-Mele model with non-Hermitian coupling. We plot the result of the full calculation by the red circles and that of the effective Hamiltonian by the purple curves. The parameters used are the same as those used in the manuscript.

Here we show an example of the effective Hamiltonian and compare it to the full calculation. For this we consider the non-Hermitian Kane-Mele model discussed in the manuscript. We use the same parameters used for Figure 2 in the manuscript, and we plot the edge bands near the crossing point in Fig. 1. The red circles are a reproduction of the edge bands in Figure 2 of the manuscript. The purple curves are the results of the effective Hamiltonian in Eq. (8). The slope of the bands is fitted from Figure 2(a) of the manuscript, i.e. the Hermitian Kane-Mele model. For this model, the effective non-Hermitian coupling strength $i\gamma'$ in Eq. (8) equals that of the bulk defined in the manuscript, i.e. $\gamma' = 0.2 \times 3\sqrt{3}\lambda_{so}$ and $\lambda_{so}$ is the second nearest neighbor coupling strength. We observe in Fig. 1 that the effective $2 \times 2$ model faithfully reproduces the edge bands near the crossing point of the full calculation.

## TOPOLOGICAL EDGE-GAIN IN BERNEVIG-HUGHES-ZHANG MODEL

In the momentum space, the Bernevig-Hughes-Zhang model [5] with a non-Hermitian coupling between the spins is written as $h(k) = h_{BHZ}(k) + \Gamma$, where

$$h_{BHZ}(k) = \begin{pmatrix} h_\uparrow(k) & 0 \\ 0 & h_\downarrow(k) \end{pmatrix}, \quad \Gamma = \begin{pmatrix} 0 & i\gamma s^x \\ i\gamma s^x & 0 \end{pmatrix} \tag{9}$$

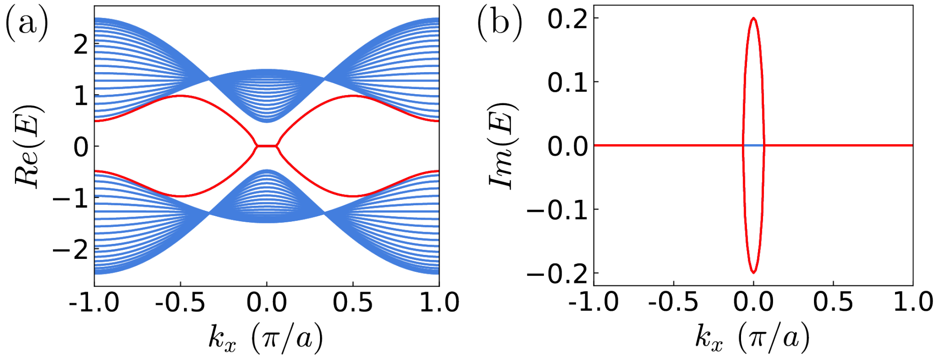


Figure 2. Calculated real (a) and imaginary (b) parts of the band structure of the Bernevig-Hughes-Zhang model with non-Hermitian couplings. The bulk bands are colored in blue, and the edge states in red.

Here, $h_{BHZ}$ is the original Bernevig-Hughes-Zhang Hamiltonian, where $h_{\uparrow}(k) = \vec{d}(k) \cdot \vec{s}$, $\vec{s} = (s^x, s^y, s^z)$ are the Pauli matrices, and $\vec{d} = (\sin k_x a_x, \sin k_y a_y, m + \cos k_x a_x + \cos k_y a_y)$. $h_{\downarrow}(k) = h^*_{\uparrow}(-k)$, as is required by time reversal symmetry. $\Gamma$ is the non-Hermitian coupling between spins.

The total Hamiltonian $h(k)$ with the non-Hermitian couplings satisfies a $\mathcal{PT}$ symmetry, where $\mathcal{P} = \sigma^z \otimes I$ is the spatial inversion, and $\mathcal{T} = I \otimes s^x K_0$ is the Bosonic time reversal, where $\sigma^i$ and $s^i$ are the Pauli matrices describing the sub-lattice and the spins, respectively, and $K_0$ is complex conjugation.

The calculated band structure of a stripe structure that is periodic in $x$ and finite in $y$ is shown in Fig. 2. For this calculation, we have set $m = 0.5$, and $\gamma = 0.2$. It is clear that with the non-Hermitian couplings, the bulk bands remain in the $\mathcal{PT}$-exact phase, while the gapless edge states enters the $\mathcal{PT}$-broken phase, showing gain.

## COUPLED MODE EQUATION

We give a derivation of Eq. (5) of the main text. Assuming the amplitude of the cw and ccw modes to be $a_1$ and $a_2$, we have [6]

$$\begin{aligned} \frac{da_1}{dt} &= -\frac{2}{\tau} a_1 + \sqrt{\frac{2}{\tau_1}} S_1^+ \\ \frac{da_2}{dt} &= -\frac{2}{\tau} a_2 + \sqrt{\frac{2}{\tau_2}} S_2^+ \end{aligned} \tag{10}$$

where $1/\tau$ is the leakage rate into the couplers from the ring. $S^{\pm}_{1,2}$ are the power moving toward (+) and away from (−) the coupling region in the coupling waveguides. They are normalized such that $|S|^2$ is the wave intensity. $S^{-}_{1,2}$ are solely caused by leakage from the main ring, and they are related to the cw and ccw modal amplitudes by

$$S_1^- = \sqrt{\frac{2}{\tau}} a_2, \quad S_2^- = \sqrt{\frac{2}{\tau}} a_1 \tag{11}$$

Additionally, we have the relations for the power in the coupling waveguide:

$$S_1^+ = S_1^- e^{i\phi_1}, \quad S_1^+ = S_1^- e^{i\phi_1} \tag{12}$$

where $\phi_{1,2}$ are the phases accumulated by waves traveling from the coupling region to the mirror and back, which can be adjusted by changing the waveguide length.

Putting together Eq. (10), (11) and (12), we arrive at the coupled mode Hamiltonian in

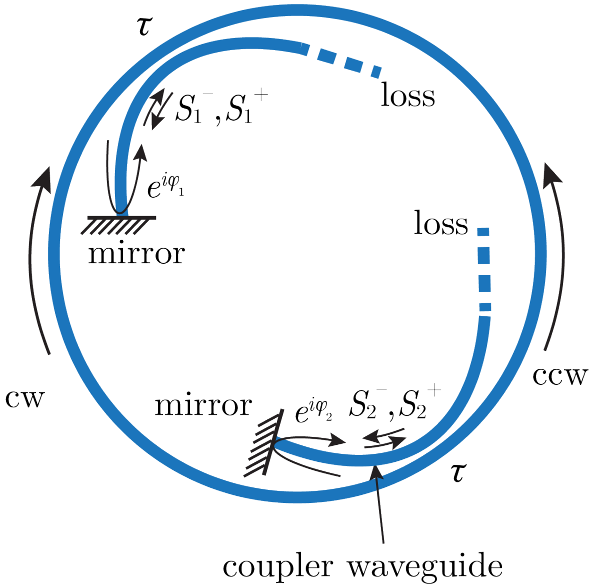


Figure 3. Schematic of a coupled ring resonator with coupling waveguides inside. Each coupler waveguide has a lossy port on one end, and is reflecting on the other end. $1/\tau$ is the leakage rate into the couplers from the ring. $\phi_{1,2}$ are the phases accumulated by waves traveling from the coupling region to the mirror and back, which can be adjusted by changing the waveguide length. $S^{\pm}_{1,2}$ are the power moving toward (+) and away from (−) the coupling region in the coupling waveguides.

Eq. (4) in the main text:

$$i\frac{d}{dt}\begin{pmatrix}a_1\\a_2\end{pmatrix}=\begin{pmatrix}-i\frac{2}{\tau} & i\frac{2}{\tau}e^{i\phi_1}\\ i\frac{2}{\tau}e^{i\phi_2} & -i\frac{2}{\tau}\end{pmatrix}\begin{pmatrix}a_1\\a_2\end{pmatrix} \tag{13}$$

## REALISTIC TOPOLOGICAL GAP AND EDGE MODAL GAIN

Here we discuss the realistic topological gap in our scheme, and the associated modal gain differential between the bulk and the edge. In recent experimental studies based on coupled ring-resonators [7–9], the reported topological gap is about $\epsilon_g = 1\,\text{nm} \approx 125\,\text{GHz}$, for a lasing wavelength of 1550 nm. Taking the Kane-Mele model with non-Hermitian coupling for example, it requires a non-Hermitian coupling strength of $\gamma = \epsilon_g/2 = 62.5\,\text{GHz}$ to close such an bulk gap, as is shown in Fig. 4(a).

We now calculate how much gain is needed to realize such a non-Hermitian coupling. For this we consider the non-Hermitian coupling matrix shown in Eq. (4) of the manuscript, reproduced here:

$$i\frac{d}{dt}\begin{pmatrix}a_1\\a_2\end{pmatrix}=\begin{pmatrix}-i\frac{2}{\tau} & i\frac{2}{\tau}e^{i\phi_1}\\ i\frac{2}{\tau}e^{i\phi_2} & -i\frac{2}{\tau}\end{pmatrix}\begin{pmatrix}a_1\\a_2\end{pmatrix} \tag{14}$$

This is the coupling matrix provided by the two waveguide couplers in a ring resonator. $a_1, a_2$ are the modal amplitude of the cw and ccw modes in the resonator, respectively. $\tau$ is the leakage rate between the ring and the coupler waveguides. $\phi_1, \phi_2$ are the phase accumulated in the coupler waveguides. The off-diagonal terms in Eq. (14) provides a non-Hermitian coupling between the cw and ccw modes, with a strength of $\gamma = 2/\tau = 62.5\,\text{GHz}$. The diagonal terms of $-i2/\tau$ represent loss to the cw and ccw modes, which is to be compensated by the pumping in the ring resonator. The loss rate is then $2/\tau = 62.5\,\text{GHz} = 0.0625\,\text{ps}^{-1}$ for the modal amplitudes, and $0.125\,\text{ps}^{-1}$ for the intensity. Assuming a group velocity of $c_0/n$ where $c_0$ is the light speed in vacuum and $n = \sqrt{12}$ is the refractive index, $0.125\,\text{ps}^{-1}$ translates into an attenuation coefficient of $14\,\text{cm}^{-1}$ in the ring. This is the modal gain required to compensate the diagonal loss term in Eq. (14) and provide the form of the non-Hermitian coupling discussed in the manuscript.

One can further increase pumping to the structure beyond this point. This will lead to gain in both the bulk and the edge. To illustrate this, in Fig. 4 we plot the band structure of the structure under a non-Hermitian coupling strength $\gamma$ of $14\,\text{cm}^{-1}$ that closes the bulk

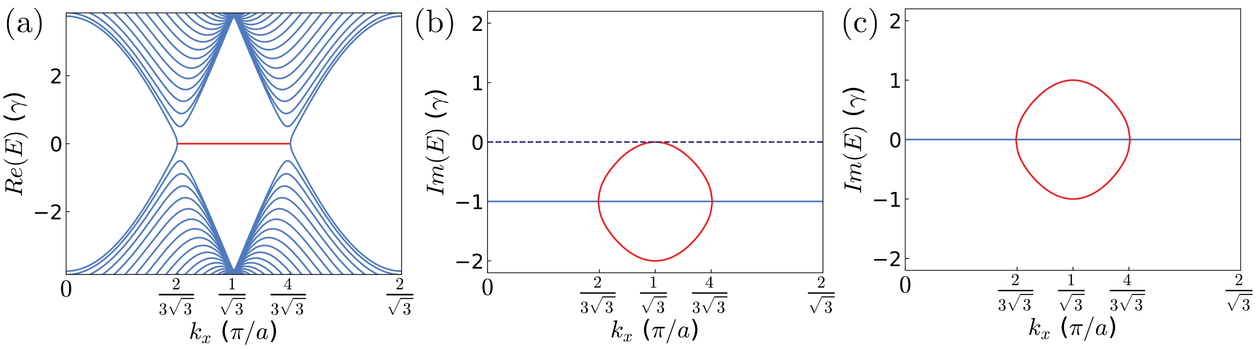


Figure 4. Band structure of Kane-Mele model with non-Hermitian coupling in a stripe geometry. All structural parameters are the same as those used in the manuscript. We choose a non-Hermitian coupling strength $\gamma = \epsilon_g/2$ at closes the bulk gap. (a) Real part of the band structure. (b) and (c) show the imaginary part of the band structure without and with pumping, respectively. Red curves represent the edge modes, while blue curves represent the bulk modes. For clarity we plot the energy in units of $\gamma$.

gap. Before pumping is applied, all of the modes in the structure are lossy with negative imaginary parts of the eigenfrequencies, except one edge mode at the wave vector of $\pi/(\sqrt{3}a)$ which is a dark mode, as is shown in Fig. 4(b). As we apply pumping to the ring resonators, the imaginary part of the eigenenergy of all modes increase. At a modal gain in the ring resonators of $14\,\mathrm{cm}^{-1}$, the bulk modes become dark, whereas the edge mode at the wave vector of $\pi/(\sqrt{3}a)$ have the highest modal gain of $14\,\mathrm{cm}^{-1}$. If we increase pumping beyond this point, modal gain will appear for bulk modes as well. However, the modal gain of the edge will always be higher than that of the bulk by $14\,\mathrm{cm}^{-1}$. Such a modal gain differential is typically sufficient for selecting lasing modes. Additional lasing dynamics including modal competition may take place, but is beyond the scope of this work.

For reference, state-of-the-art semiconductor quantum-well laser waveguides provide a modal gain of less than $50\,\mathrm{cm}^{-1}$ [9]. We note that the 1 nm topological gap reported before is for proof-of-principle experiments, and is by no means optimized. This number can be tuned by changing the coupling strength between the ring-resonators. By increasing the topological gap, one can increase the modal gain differential between the edge and the bulk.

* shanhui@stanford.edu

[1] Ali Mostafazadeh, “Pseudo-Hermiticity versus PT-symmetry III: Equivalence of pseudo-Hermiticity and the presence of antilinear symmetries,” Journal of Mathematical Physics **43**, 3944–3951 (2002).

[2] Ruili Zhang, Hong Qin, and Jianyuan Xiao, “PT-symmetry entails pseudo-Hermiticity regardless of diagonalizability,” Journal of Mathematical Physics **61**, 012101 (2020).

[3] Sean Nixon and Jianke Yang, “All-real spectra in optical systems with arbitrary gain-and-loss distributions,” Physical Review A **93**, 031802 (2016).

[4] Petr Siegl, “The non-equivalence of pseudo-Hermiticity and presence of antilinear symmetry,” Pramana **73**, 279–286 (2009).

[5] B. A. Bernevig, T. L. Hughes, and S.-C. Zhang, “Quantum Spin Hall Effect and Topological Phase Transition in HgTe Quantum Wells,” Science **314**, 1757–1761 (2006).

[6] Herman A Haus, *Waves and Fields in Optoelectronics* (Prentice Hall, 1984) pp. 1–402.

[7] Gal Harari, Miguel A. Bandres, Yaakov Lumer, Mikael C. Rechtsman, Y. D. Chong, Mercedeh Khajavikhan, Demetrios N. Christodoulides, and Mordechai Segev, “Topological insulator laser: Theory,” Science **359**, eaar4003 (2018).

[8] Miguel A. Bandres, Steffen Wittek, Gal Harari, Midya Parto, Jinhan Ren, Mordechai Segev, Demetrios N. Christodoulides, and Mercedeh Khajavikhan, “Topological insulator laser: Experiments,” Science **359**, eaar4005 (2018).

[9] Hossein Hodaei, M.-A. Miri, Matthias Heinrich, Demetrios N Christodoulides, and M. Khajavikhan, “Parity-time-symmetric microring lasers,” Science **346**, 975–978 (2014).
